# Supplementary material for: Bayesian Inference for Correlated Human Experts and Classifiers
Source: arXiv:2506.05636 source file (2025-06-05)
Supplement: Supplementary file 1 [file additional_theoretical_results.tex]

\section*{Appendix B: Theoretical Analysis of Random Expert Selection}
\label{sec:appdxb}

To better understand our experimental results, we first analyze from a theoretical perspective the achievable reduction in error for any systematic querying method, relative to a simple baseline of random querying. Questions of a similar nature have been addressed in prior work in the context of predicting the winner of an election given a random sample of votes from the full set of voters \citep{dey2015sample,micha2020can,imber2021probabilistic,bhattacharyya2021predicting}. This work often focuses on complexity analyses and asymptotic bounds involving relatively large numbers of votes (experts) in the context of a single election. Here our focus is somewhat different, on exact results for relatively small numbers of experts, e.g., as few as $N=3$, motivated by practical considerations on typical availability of expert opinion. In addition,  we are interested in average performance over multiple ``elections,'' where in our setup each example  $x$  corresponds to a different ``election'' with potentially different voting patterns across such elections. 

Below we introduce some basic lemmas (and corresponding proofs) whose results provide some insight into the performance of random querying. We refer to these theoretical results in our discussion of experimental results in the main paper.
 
Consider $H$ experts and $K$ classes. For any particular example $x$ each expert will map $x$ to a label, resulting in a consensus label $y_*$ for the group (the labeling can be deterministic---i.e., always the same label for an expert given the same $x$---or stochastic). 
Assume for simplicity that the consensus label $y_*$ always is unique (i.e., no ties in voting); this will always be satisfied for example if $K=2$ and $N$ is odd.

For any example $x$, let $n_c$ be the size of the {\it consensus set}, defined as the number  of experts that vote for the consensus $y_*$, with $H-n_c$ experts voting for other labels $y_k \ne y_*$. (For simplicity the dependence on $x$ is implicit in notation for $n_c$ and $y_*$.) Given some underlying distribution $p(x)$, this induces a distribution over the sizes of consensus sets, namely $p(n_c)$, with $ \lceil \frac{H}{K} \rceil \le n_c \le H$.

\paragraph{Random Querying of 1 or 2 Experts:}
Consider the strategy where for each $x$ we query uniformly at random a subset of $n_q$ experts from the set of total experts and use the consensus $\hat{y}_*$ (with ties broken randomly) of the subset to predict the unobserved true consensus.
Of interest is the average error $Err$ of using $\hat{y}_*$ to predict $y_*$.   
\begin{lemma}
    Querying either one or  two randomly selected experts results in an error rate $Err = 1 - \frac{E[n_c]}{H}$, where the expectation $E$ is with respect to $p(x)$ or equivalently to $p(n_c)$.
\end{lemma}  
Intuitively this makes sense: the larger the consensus set is on average,  the more likely it is that 1 (or 2) randomly selected experts will generate the correct consensus prediction.

\paragraph{Proof of Lemma 1: Case 1, $n_q=1$:}
With $n_q=1$, for each $x$,  there are two possible outcomes:
\begin{enumerate}
\item The queried expert is in the consensus set with probability $p_c = n_c/H$ and the error at $x$ is 0.
\item The queried expert is in the non-consensus set with probability $1- p_c = 1 - n_c/N$ and the error at $x$ is 1, since by definition if the selected expert is not in the consensus set then their prediction disagrees with the consensus.
\end{enumerate}

Thus,  for any specific $x$ and specific $n_c$, $Err_x = 0 p_c  + 1 (1-p_c) = 1-p_c$.
Averaging wrt $p(x)$,  we get 
\begin{eqnarray*}
    Err & = &  \int_x p(x) (1-p_c) dx  = \sum_{n_c}  p(n_c) (1-p_c) \\
    & = & \sum_{n_c}  p(n_c) (1 - n_C/H)  \\
    & = & 1 - \sum_{n_c}  p(n_c) (n_C/H) \\
    & = &1 - \frac{E[n_c]}{H}. 
\end{eqnarray*}  
 Or,  equivalently,  the accuracy of random querying with a single expert is $Acc = E[n_c]/H$.

\paragraph{Proof of Lemma 1: Case 2 $n_q=2$:} When querying 2 randomly selected experts.
there are 4 possible outcomes, denoted as $CC,  CI, IC,  II$ where $C$ indicates an expert in the consensus set (making a correct prediction) and $I$ indicates an expert in the non-consensus set (making an incorrect prediction).  

The order of $IC$ and $CI$ does not matter for making predictions, in effect reducing the outcomes to 3:
\begin{enumerate}
\item CC: the first 2 experts are in the consensus set.  This outcome has error 0 and occurs with probability $\frac{n_c}{H} \frac{n_c -1}{H-1}$.
\item II: the first 2 experts are both in the non-consensus set.  This outcome has error 1 and occurs with probability $\frac{H-n_c}{H} \frac{H-n_c -1}{H-1}$.
\item CI or IC.  Each of these two outcomes has the same probability $\frac{n_c}{H} \frac{H-n_c}{H-1}$, with a total outcome probability of $2  \frac{n_c}{N} \frac{H-n_c}{H-1}$.   Since one vote $C$ is consensus and the other is not, this outcome is a tie between the correct consensus label and some other label.  Ties are broken randomly leading to an error rate of 0.5
\end{enumerate}

Thus,  the overall error rate,  for any specific $x$ and corresponding $n_c$ is
\begin{eqnarray*}
Err_x & = & 0 + 1 \frac{H-n_c}{H} \frac{H-n_c -1}{H-1} + 2  \frac{n_c}{H} \frac{H-n_c}{H-1} 0.5\\
& = & (H-n_c) \frac{H- n_c - 1 + n_c}{H(H-1)}\\
& = & (H-n_c) \frac{H-1}{H(H-1)}\\
& = & 1 - \frac{n_c}{H}
\end{eqnarray*}
Averaging over $p(x)$ as before yields the desired result.

\paragraph{Random Querying for General Numbers of Experts:}
For $n_q > 2$ there are a combinatorial number of options to consider, making a direct analysis of the error rate difficult and likely to not be insightful. Nonetheless, we can make some progress under certain assumptions.
\begin{assumption} 
$p[n_c] = 0 $ for $n_c \le \lfloor \frac{H}{2} \rfloor$ (strict majority)
\end{assumption}
\begin{assumption} 
All the $H-n_c$ non-consensus votes are for the same particular class label $k \ne k^*$ where $k^*$ is the consensus label.
\end{assumption}
Assumption 2 is adversarial in the sense that all of the non-consensus experts agree on the same label, a label $k$ that is different to the consensus label. Both assumptions are true trivially for $K=2$.

\begin{lemma}
    Under assumptions 1 and 2, for odd values of $n_q$, querying $n_q$ randomly selected experts results in an error rate $Err =  \sum_{n_c} p(n_c) Err_{n_c}$, where  $Err_{n_c} = F_{HG}(r; H, n_c, n_q)$ and $ F_{HG}( )$ is the  hypergeometric cumulative distribution function   with argument $r = \lfloor \frac{n_q}{2} \rfloor$ and parameters $H$ (total number of experts), $n_c$ (number of experts in the consensus set), and $n_q$ (number of samples drawn without replacement from the  $H$ experts). 
\end{lemma} 

\noindent{\bf Simple Example:} Let  $H=10$ and $n_c=6$. For querying with  $n_q = 1, 3, 5, 7, 9$ random experts we get error rates (from the CDF) of $40.0, 33.3, 26.19, 16.67, 0.00$ respectively.  The value for $n_q=1$ is trivial: we have a $4/10$ chance of picking a non-consensus expert. Note that even if we query a relatively large number of  $n_q=7$ experts, the error rate is still non-zero (and relatively high) since there is a chance that we get all 4 non-consensus experts and 3 of the 6 consensus experts. This reinforces the earlier idea that the further away $n_c$ (and $E[n_c]$) is from $H$, i.e., the weaker the consensus, the higher the error rates of random querying and there is (correspondingly) more opportunity for reducing the error rate via systematic (e.g., model-based) querying.

\paragraph{Proof of Lemma 2}

For any $x$ and a set of associated expert labels, under assumption 2 there are two possible labels that have a non-zero number of votes: the consensus label $k^*$ and a second non-consensus label $k \ne k^*$. Thus, in sampling $n_q$ votes, we are in effect sampling without replacement from an urn with $N$ total items, where $n_c$ of them have one color and $N-n_c$ have another color (out of a total of $K$ possible colors). This can be modeled as a hypergeometric distribution, which we can use to compute the probability of obtaining $r$ consensus labels if we draw $n_q$ samples from an ``urn" which contains $n_c$ consensus labels (``balls" of one color) and $N-n_c$ non-consensus labels (``balls" of a different color). 

If we use the random sample to predict the true consensus, we will make an error whenever our sample contains fewer consensus labels than non-consensus labels (assuming for simplicity we draw an odd number $n_q$ of samples). The probability of this happening is the sum of probability masses for outcomes of the hypergeometric distribution for arguments $r=0, 1, \ldots, \lfloor \frac{n_q}{2} \rfloor$, i.e., the sum of probabilities that we get fewer consensus labels in our sample than non-consensus labels.  This sum is the CDF (left tail) of the hypergeometric distribution with argument $\lfloor \frac{n_q}{2} \rfloor$ and parameters $N, n_c$ and $n_q$.

To complete the proof, note that the error above is for any fixed value of $n_c$. Since $n_c$ is random wrt $p(n_c)$ we take the expectation with $p(n_c)$ to get the overall average error rate across all $x$.

\paragraph{Expert Correlation and Random Querying}
The results above focus on error as it depends on expected consensus set size. We can also analyze error as a function of a related quantity---the correlation between expert predictions.
Consider the special case of $K=2$ classes and $N$ experts, where we consider a single real-valued logit $z_i$ for each expert $i=1,\ldots,H$. The vector ${z} = (z_1,\ldots,z_H)$ is a random variable driven by the variation in $p(x)$. Assume a multivariate normal distribution for the ${z}$ with mean $\mu_z = 0$ and some covariance $\Sigma_z$.  Labels are generated in the following manner: if $z_i > 0$ then expert $i$ produces a class label of 1, and otherwise a label of 0.

The probability that any particular vote vector  occurs, out of the $2^H$ possible binary vote vectors, can be computed by determining how much probability mass is in the corresponding  orthant. Unfortunately these orthant probabilities for multivariate Gaussians are not available in closed form in general (e.g., see \cite{ridgway2016computation}). Nonetheless, consider the special case of equicorrelation:  $\Sigma$ has $\sigma_{ii} = 1$ and   all off-diagonal correlations are constant and non-negative with $\rho_{i,j} = \rho \ge 0, i \ne j$. Under these assumptions, there are simple closed form expressions (e.g.,  \cite{abrahamson1964orthant}) for orthants  for the cases of $N=2, 3, 4$, allowing for statements such as the following:
\begin{lemma}
    Given the equicorrelated Gaussian model above, for $K$=2 classes and $H=3$ experts, the error rate of randomly querying either 1 or 2 experts can be expressed as
    \[
    Err  \ = \  1 - \frac{ E[n_c] }{3} \ = \  0.25 - \frac{\arcsin(\rho)}{2\pi}  \ < \  0.25 - \frac{ \rho }{2\pi},
    \]
\end{lemma} 
i.e., the error is bounded above by a function that decreases linearly as a function of expert correlation, and in the exact expression we see that $Err$ changes from 0.25 to 0 as $\rho$ ranges from 0 to 1. Expressions for $H=4,5,\ldots$ experts are attainable but lack the simplicity of the result above for $N=3$.

\paragraph{Proof of Lemma 3}
The orthant probability of a vote vector of all 1's or all 0's, for an equicorrelated Gaussian model in $H=3$ dimensions can be written as
\[
P_3 = \frac{1}{8} + \frac{3}{4\pi} \arcsin{\rho}
\]
(e.g., see \cite{abrahamson1964orthant}), and the probability of getting a vote with consensus strength $n_c=3$  is $2 P_3$.

The probability of generating a vote vector in one of the other 6 orthants must be $1-2P_3$: and in each of these orthants there must be   2 votes that agree and 1 that is different: so the consensus strength $n_c$ in these 6 orthants is 2.

Thus,
\begin{eqnarray*}
E[n_c]  & = &  2 \times (1 - 2P_3)  + 3 \times 2 P_3  \\
    & = & 2 + 2 P_3  
\end{eqnarray*} 
and we know from Lemma 1 that $1 - E[n_c]/H$ is the error rate for random  querying of 1 or 2 experts. Hence,
\[
Err = 1 - \frac{1}{3}(2 + 2 P_3) = 0.25 - \frac{\arcsin{\rho}}{2\pi}.
\]
 The inequality in Lemma 3 is from a standard bound on $\arcsin$ in the range $x\in [0,1]$ (e.g., \cite{bagul2021simple})
 \[
 1 + \frac{x^2}{6} < \frac{\arcsin(x)}{x} < 1 + \frac{\pi - 2}{2}x^2
 \]

Although the results above are for relatively simple cases, they nonetheless confirm our intuition about what should ``drive''  error rates of random querying, namely distributional properties of how often experts agree, driven in turn by how correlated the experts tend to be. In turn, these factors provide bounds on what is achievable beyond random querying, as we will see in our experiments.
